# Supplementary material for: Study of vacancy ordering and the boson peak in metastable cubic Ge-Sb-Te using machine learning potentials
Source: arXiv:2309.01089 source file (2024-01-04)
Supplement: Supplementary file 1 [file Supplemental_Material.pdf]

**Supplemental Material for: Study of vacancy ordering and the boson peak in metastable cubic Ge-Sb-Te using machine learning potentials**

Young-Jae Choi, Minjae Ghim, and Seung-Hoon Jhi*

*Department of Physics, Pohang University of Science and Technology, Cheongam-ro 77, Pohang 37673, Republic of Korea*

*e-mail: *jhish@postech.ac.kr*

**Table S1. RAG dataset composition of GST225 potential.** The main data (64650 frames) are highlighted in yellow. The item "random_frac" is an input parameter for RAG scripts. The (A×B) format in the "Num. frames" column means A (the number of RAG random configurations) times B (the number of structure relaxation steps for each RAG random configuration). The "Energy and Force RMSE" columns denote the root-mean-squared errors of corresponding datasets. The last-row class "etc (RAG)" is for the remaining data including the single-element (Ge/Sb/Te) systems and some segregated structures for example.

| **Target** | **Backbone structure** | **Size** | **random _frac** | **Num. frames** | **Energy RMSE** (meV/atom) | **Force RMSE** (meV/Å) |
|---|---|---|---|---|---|---|
| Hexagonal states (ground states) | Kooi supercell | 81 atoms | 0 | 100 copies | 55.7 | 2.62 |
| | Petrov supercell | 81 atoms | 0 | 100 copies | 29.9 | 3.90 |
| | Inverted Petrov supercell | 81 atoms | 0 | 100 copies | 42.2 | 12.0 |
| | Ferro-GeTe supercell | 81 atoms | 0 | 100 copies | 36.5 | 9.66 |
| | Inv.-Fer. supercell | 81 atoms | 0 | 100 copies | 32.1 | 8.95 |
| | Petrov-Fer. supercell | 81 atoms | 0 | 100 copies | 30.0 | 10.3 |
| Kooi phase (thermally excited states) | Kooi unit cell | 9 atoms | 0.02 | 200 | 55.5 | 7.18 |
| | | | 0.1 | 200 | 55.7 | 32.0 |
| | Kooi supercell | 144 atoms | 0.02 | 177 | 55.4 | 5.00 |
| | | | 0.1 | 185 | 55.4 | 22.0 |
| Matsunaga and VOC | Six hexagonal supercells | 81 atoms | 0.25 | 1350×10 =13500 | 42.3 | 43.9 |
| Rock-salt cubic phase | Rock-salt FCC supercell | 57 atoms | 0.3 | 1064×15 =15960 | 33.8 | 43.8 |
| Amorphous solid | | | 0.7 | 1256×15 =18840 | 41.7 | 95.8 |
| Liquid or more | | | 0.8 | 1050×15 =15750 | 32.5 | 103 |
| etc (RAG) | - | - | - | 1045 | 501 | 139 |
| Total | - | - | - | 66,457 | 49.0 | 75.0 |

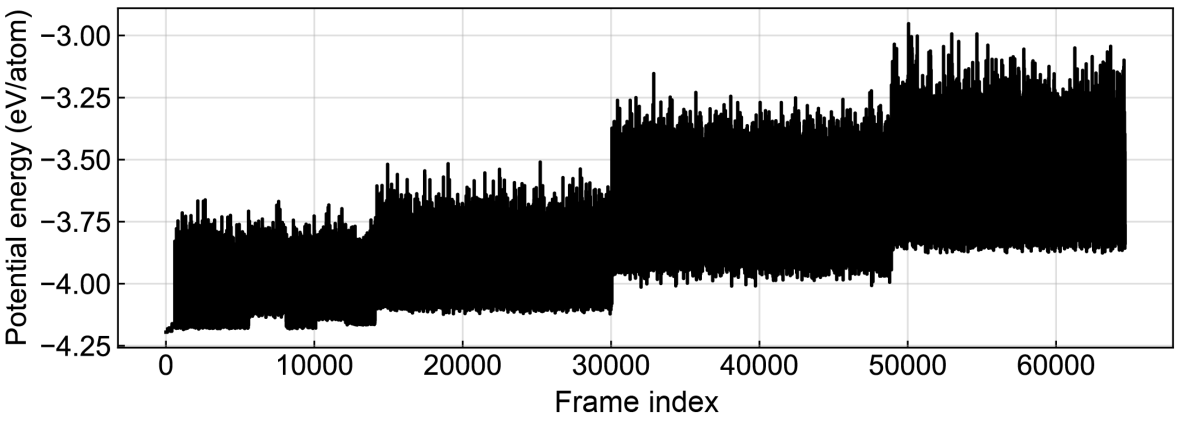


**Fig. S1. The potential energy plot of the main RAG dataset.** The composition of the main dataset is described in Table S1.

**Table S2. NequIP training parameters used to produce GST225 potential.**

<table>
<tr><td>NequIP version</td><td>0.5.3</td><td colspan="2">learning_rate</td><td>2.e-3</td></tr>
<tr><td>r_max</td><td>4.0</td><td colspan="2">batch_size</td><td>5</td></tr>
<tr><td>l_max</td><td>3</td><td rowspan="3">loss_coeffs</td><td>forces</td><td>1.e+3</td></tr>
<tr><td>num_layers</td><td>5</td><td rowspan="2">total_energy</td><td rowspan="2">1<br>PerAtomMSELoss</td></tr>
<tr><td>num_features</td><td>8</td></tr>
<tr><td>parity</td><td>false</td><td colspan="2">optimizer_name</td><td>adam</td></tr>
<tr><td>nonlinearity_type</td><td>gate</td><td colspan="2">lr_schedular_name</td><td>ReduceLROnPlateau</td></tr>
<tr><td>num_basis</td><td>8</td><td colspan="2">lr_schedular_patience</td><td>1</td></tr>
<tr><td>polynomialCutoff_p</td><td>6</td><td colspan="2">lr_schedular_factor</td><td>0.6</td></tr>
<tr><td>invariant_layers</td><td>2</td><td colspan="2">default_dtype</td><td>float32</td></tr>
<tr><td>invariant_neurons</td><td>64</td><td colspan="2">seed</td><td>123</td></tr>
<tr><td>use_sc</td><td>true</td><td colspan="2">dataset_seed</td><td>456</td></tr>
</table>

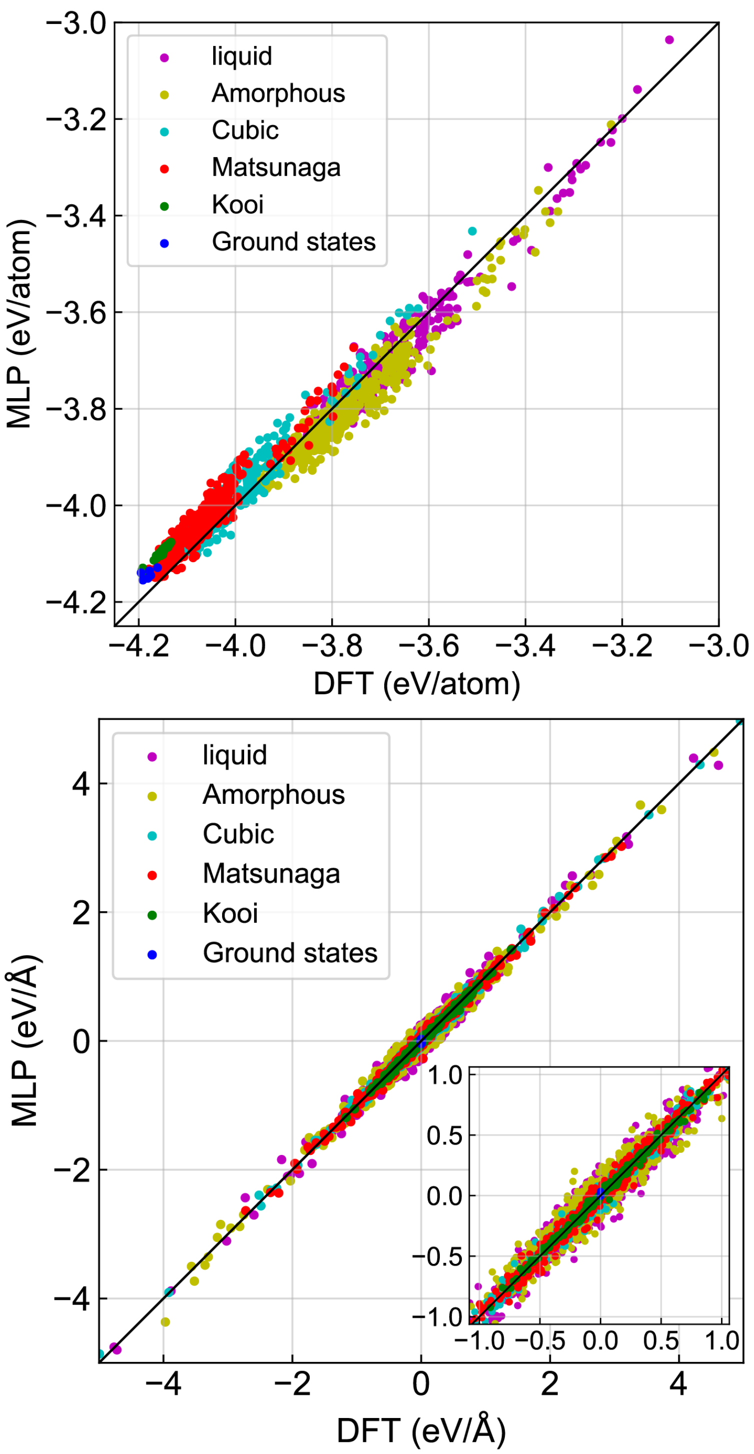


**Fig. S2. Comparison of energy (upper panel) and force (lower panel) calculations between VASP (DFT) and NequIP (MLP).**

## Validation of GST225 potential

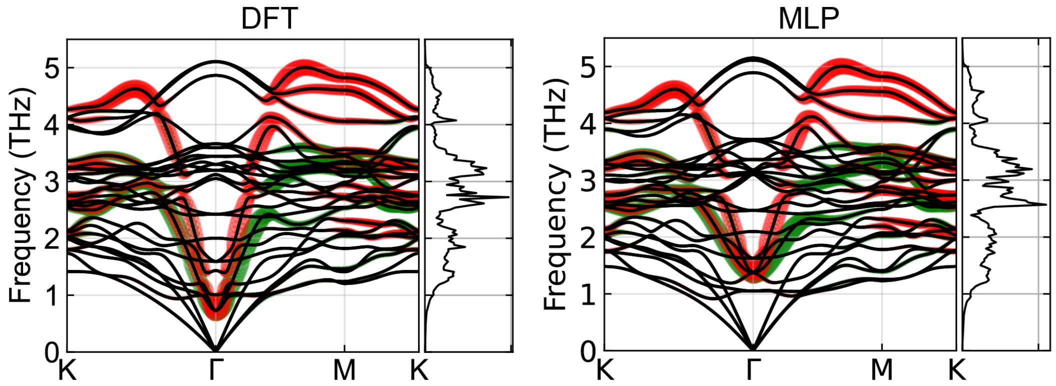


**Fig. S3. Phonon band structure of Kooi phase calculated by VASP (DFT) and NequIP (MLP) potentials of GST225.** Two narrow panels attached to the right side of phonon band plots are phonon density of states. The similarity of each mode to the $E_u$ modes is expressed by green ($E_u$-A mode) and red ($E_u$-B mode) highlights. The thickness of highlights is proportional to the squared inner product of two modes $\sim\left|\boldsymbol{\varepsilon}\cdot\boldsymbol{\varepsilon}_{E_u-\mathrm{A,B}}\right|^2$. $E_u$ mode is a characteristic optical phonon mode of hexagonal GST, which is very sensitive to strain [1].

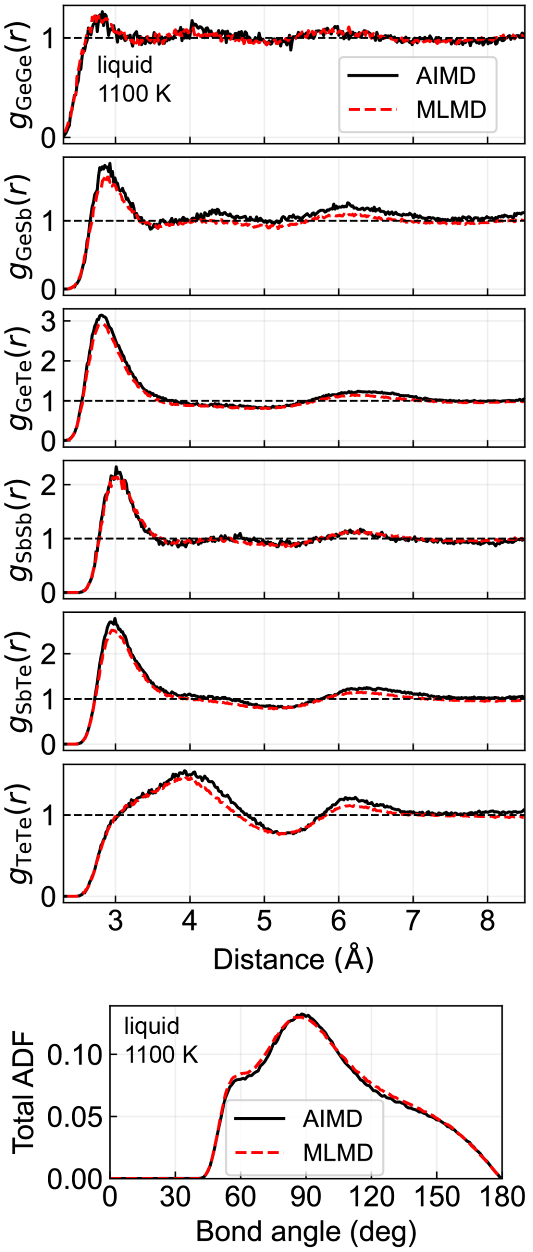


**Fig. S4. Comparison of partial RDFs (top panel) and total ADFs (bottom panel) liquid GST225 at 1100 K.** The AIMD simulation conditions: 54 atoms in a frame; NpT (p=0). The MLMD simulation conditions: 10368 atoms in a frame; NVT ensemble (0.0309 atoms/Å$^3$, the same density as the NpT ensemble).

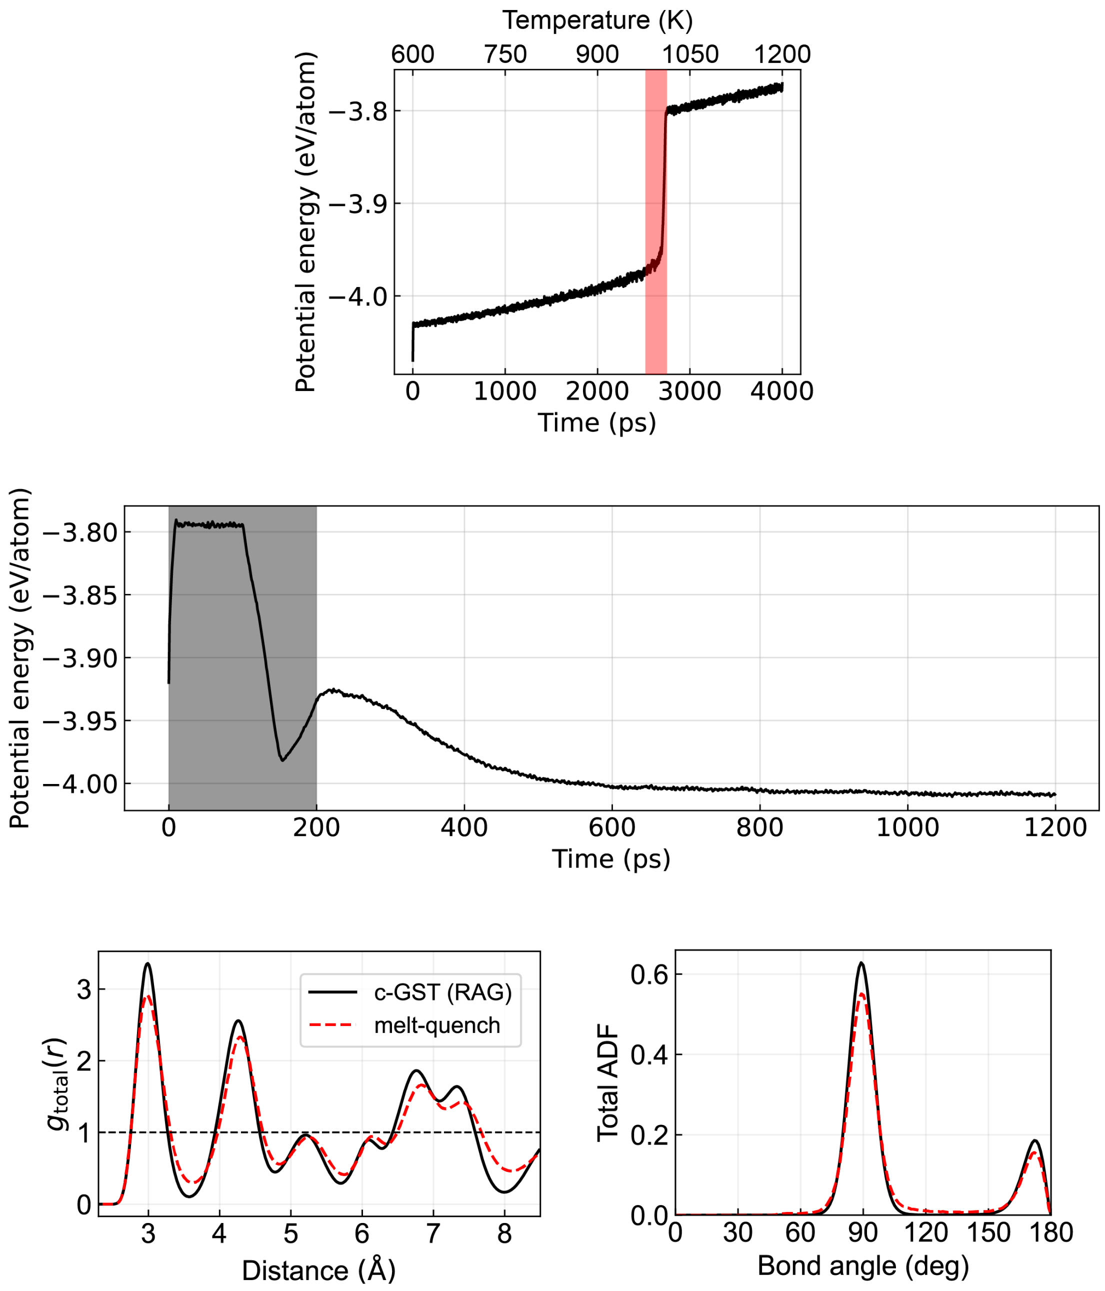


**Fig. S5. Potential energy change of GST225 during melting (upper panel) and amorphous-to-cubic crystallization (middle panel).** Bottom panel shows the comparison of RDFs and ADFs between the final structure of the crystallization (dashed line in red labeled melt-quench) and the c-GST structure from the annealing simulation discussed in the main manuscript (solid line in black labeled c-GST (RAG)). The heating rate in the melting simulation was 0.15 K/ps. In the upper panel, a red transparent box (975-1015 K) highlights the temperature range where the energy changes drastically. In the middle panel, a grey

transparent box (0-200 ps) marks the preparation step, which includes the melt-quenching and heating (melting at 1100 K for 0-100 ps, quenching to 300 K for 100-150 ps, and heating to 600 K for 150-200 ps).

## RDF and ADF of c-GST at 700 K

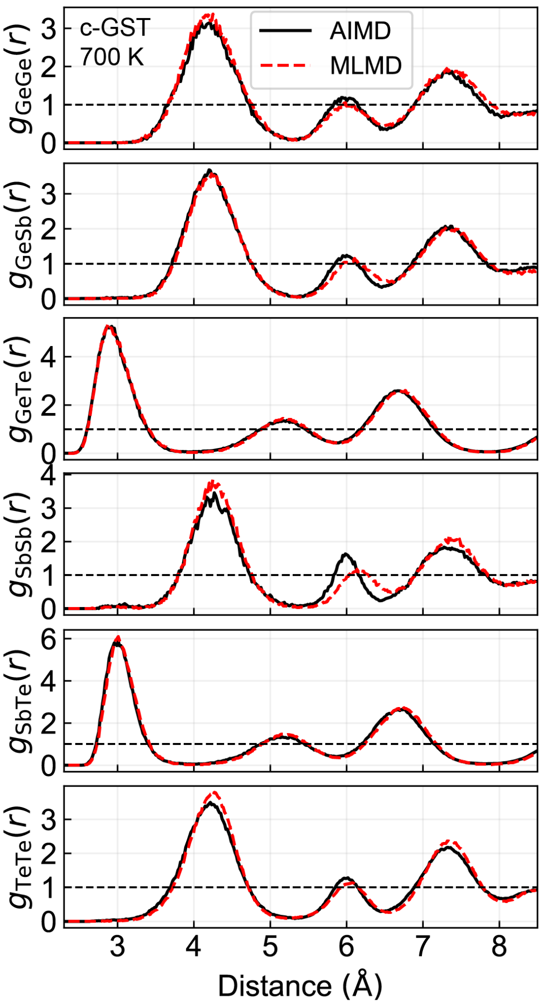


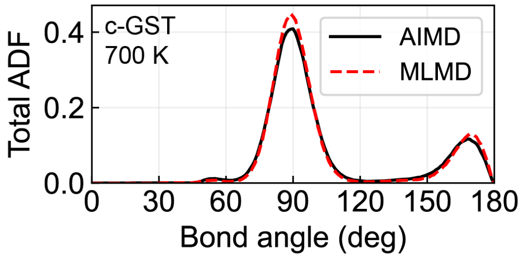


**Fig S6. Partial RDFs (top panel) and total ADFs (bottom panel) of c-GST at 700 K.** For MLMD plots, 10 intermediate atomic configurations between 0~100 ps of annealing simulation were used. The AIMD simulation conditions: 57 atoms in a frame; NVT (0.0331 atoms/Å$^3$, the same density as the MLMD simulation).

**An example of the vacancy configuration of c-GST**

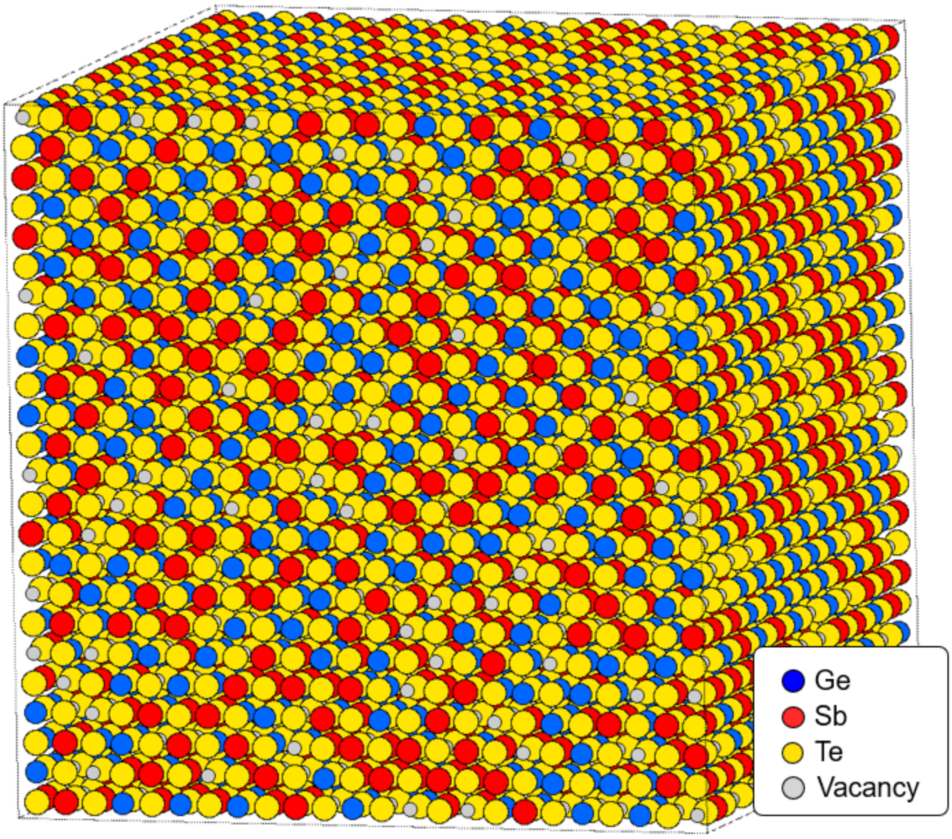


**Fig. S7. The visualization of the initial RAG configuration including vacancies.** The system contains 1382 vacancies (gray spheres) randomly arranged at cation sites. The algorithm used to find vacancies is described in the computational details section in the main manuscript.

**RDF and ADF changes in annealing simulation**

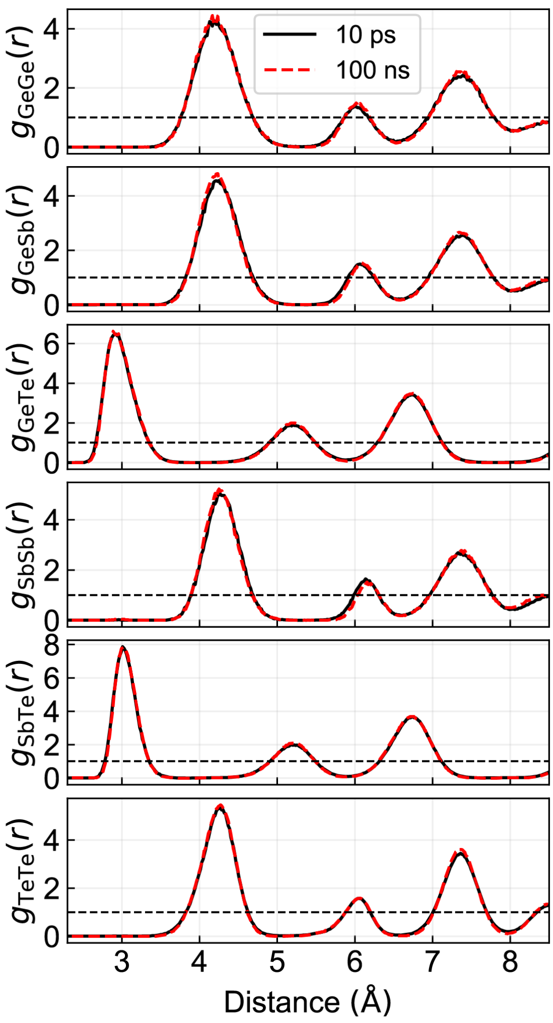


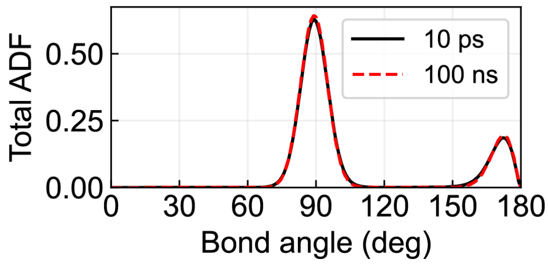


**Fig. S8. Comparison of partial RDFs (top panel) and total ADFs (bottom panel) of c-GST annealed for 10 ps (solid line in black) and 100 ns (dashed line in red).** To calculate RDFs and ADFs, the NVT (300 K) simulations were carried out the same way as for VDOS calculations in Fig. 7.

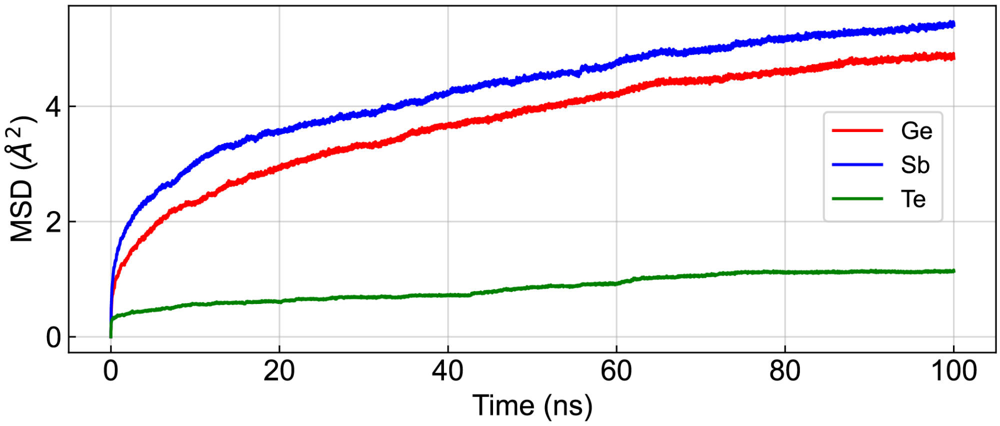


**Fig. S9. Species-wise mean squared displacement along the annealing.** The reference positions for the displacement measurement are the coordinates of the initial RAG configuration at 0 s of annealing.

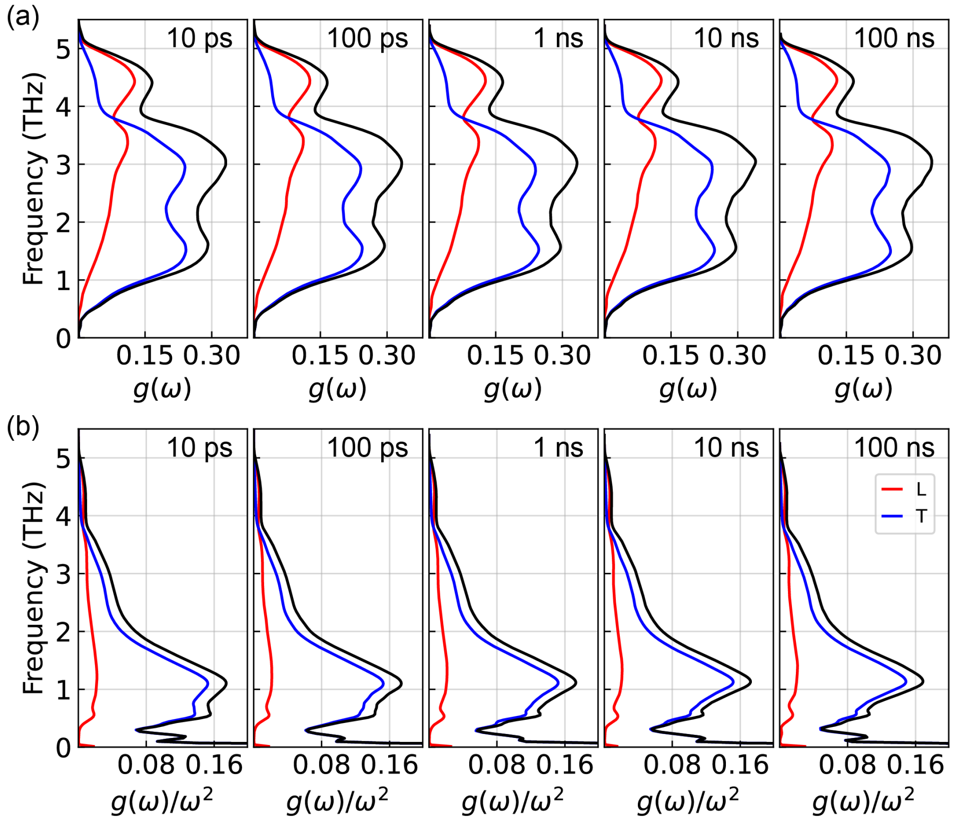


**Fig. S10. Longitudinal-transverse decomposition of VDOSs based on the Voronoi cell method.** Blue solid lines (labeled "T") and red solid lines (labeled "L") indicate the transverse and longitudinal modes, respectively. The decomposition into transverse and longitudinal mode is based on the Voronoi cell method introduced by Beltukov *et al*. [2].

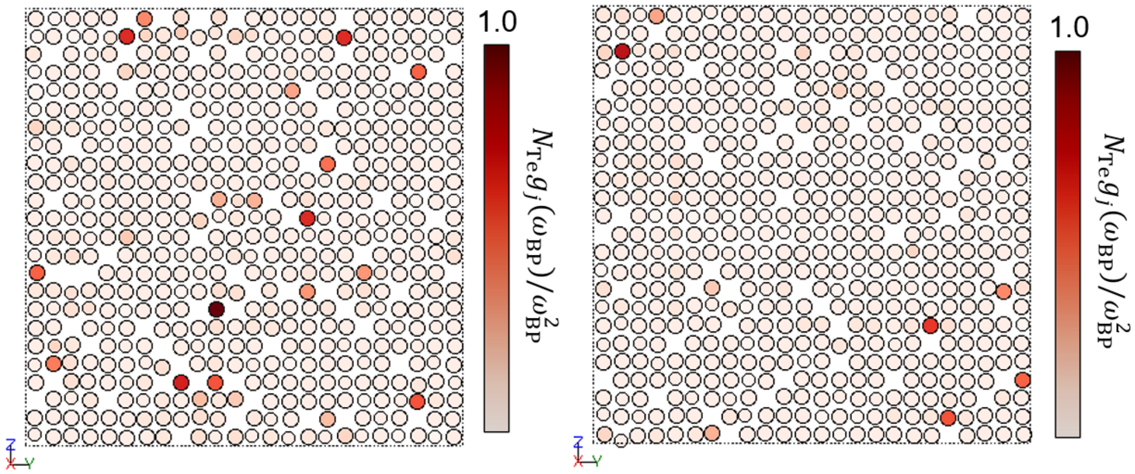


**Fig. S11. Examples of the atom-wise intensity of the boson peak modes.** The color of an atom indicates the atom-wise intensity of the vibrational modes with frequency 0.375~0.775 THz The visualized 2-dimensional atomic configurations are the single-layer slices extracted from the 10 ps configuration of c-GST annealing.

## Structure and VDOS of c-GST directly crystallized from a-GST

The RAG configuration was chosen as the initial structure for the annealing simulation instead of the c-GST configuration directly crystallized from a-GST since the latter has a more disordered Te lattice structure. The initial RAG configuration was found to be similar to the c-GST structure crystallized from a-GST, as demonstrated by the *p*-bonding chain length distribution and VDOS analyses (Fig. S12). The directly crystallized structure also displayed a power-law-like distribution of the *p*-bonding chain lengths, similar to the RAG configuration of Fig. 3a, but had a significant number of the odd-length *p*-bonding chains due to the distortion of the Te lattices. The VDOS of the directly crystallized structure at 300 K also showed a boson peak at ~0.560 THz, which was broadened by a 500 ps-long annealing process and the distortion of the Te lattices.

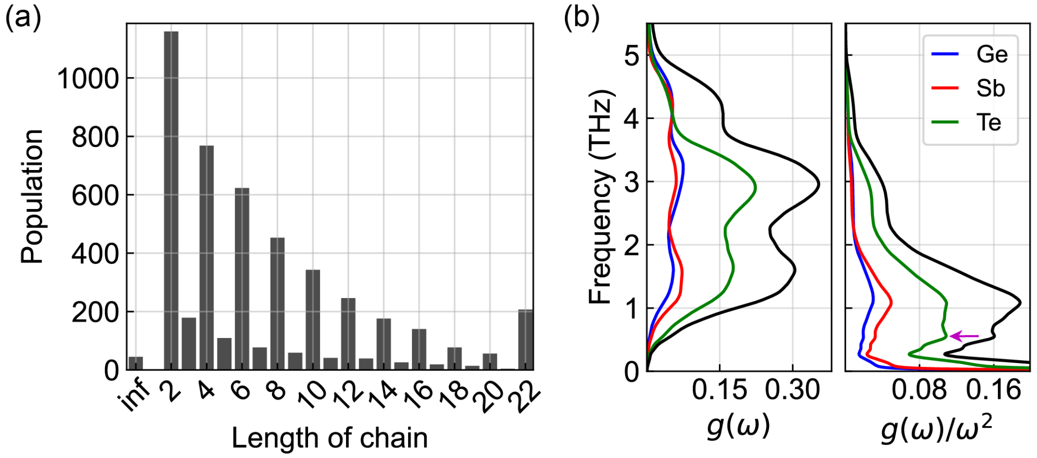


**Fig. S12. The (a) *p*-bonding chain length histogram and (b) VDOS calculated by VACF of c-GST at 300 K crystallized from a-GST.** A melt-quenched a-GST was crystallized by heating of 200 ps long from 300 K to 700 K followed by annealing of 300 ps long at 700 K and cooling of 50 ps long to 300 K. A c-GST seed consisting of 2053 atoms was attached to a-GST to aid single-domain crystallization. An equilibrium NVT-MD (300 K) was simulated to calculate VDOS in (b). The purple arrow in (b) highlights the boson peak at 0.560 THz.

**Lattice thermal conductivity calculated by Müller-Plathe rNEMD simulation**

The lattice thermal conductivity of c-GST with various vacancy distributions was calculated using the reverse nonequilibrium molecular dynamics (rNEMD) method. This rNEMD method is based on the macroscopic definition of thermal conductivity $J_x = -\kappa_{xx}\frac{\partial T}{\partial x}$, where $J_x$ is the heat current, $\kappa_{xx}$ is a diagonal component of the lattice thermal conductivity tensor, and $\partial T/\partial x$ is the temperature gradient along the $x$-axis. In this approach, the lattice thermal conductivity is obtained from the ratio of the thermal gradient to the manually built heat current. The Müller-Plathe method is a simple and powerful rNEMD algorithm that satisfies the necessary conditions for steady-state ensembles, especially the laws of energy and momentum conservation [3].

The simulation box was evenly partitioned into $2N$ slabs in the direction of interest, with the momentum of the hottest atom in the first slab and the coldest atom in the $(N + 1)$-th slab being exchanged periodically with a constant time interval [3]. When a steady state is established by the thermal flux inside the simulation box and manual energy exchange after a long enough simulation, the lattice thermal conductivity can readily be calculated [3]. The rNEMD simulations based on the Müller-Plathe method in this study were implemented using the LAMMPS package [4].

We investigated the effect of vacancy ordering in c-GST on lattice thermal conductivity. We chose the configurations at 10 ps and 100 ns and calculated the lattice thermal conductivity using 300 K rNEMD simulations. The configurations at 10 ps and 100 ns were partitioned into 24 equal-sized slabs along the $x$-direction. The virtual heat flux was established by cooling the first slab as a heat sink at –4 eV/ps and heating the thirteenth slab as a heat source at 4 eV/ps. An initial 50 ps-long rNEMD simulation was conducted to establish a steady state with the virtual heat flux, followed by a 1 ns-long rNEMD simulation, from which the temperature profile was sampled (Fig. S13). The temperature gradient was calculated using the least-square regression function from the SciPy package [5] in the regions showing linear temperature slopes (slabs 4~10 and 16~22, Fig. S13). The lattice thermal conductivities calculated by the non-stochastic rNEMD method were 0.41 W/mK and 0.40 W/mK for the 10 ps and 100 ns configurations, respectively. This result indicates that lattice thermal conductivity in c-GST is insensitive to vacancy distribution, which is consistent with experimentally indistinguishable

lattice thermal conductivities between c-GST and h-GST [6-9]. The room-temperature lattice thermal conductivities of c-GST and h-GST were measured as 0.4~0.5 W/mK [6-9]. The lattice thermal conductivity of h-GST is high in the in-plane direction but low in the out-of-plane direction due to the periodic array of vdW gaps [10]. As a result, the average lattice thermal conductivity of h-GST is similar to that of c-GST with a complex vacancy distribution. Our calculated lattice thermal conductivity using the Müller-Plathe method was 0.42 W/mK for both the 10 ps and 100 ps configurations.

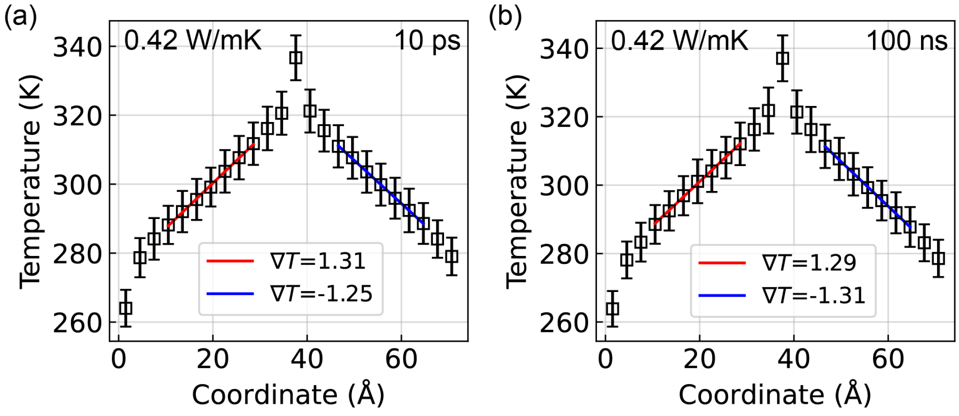


Fig. S13. Temperature profile along the *a*-direction of (a) 10 ps and (b) 100 ns configurations from 300 K Müller-Plathe rNEMD simulations. The vertical bars indicate the standard deviation of slab temperatures for 1 ns, where the slab temperature at a time point was measured every 1 ps by averaging temperatures of the past 1 ps. The coldest atom in slab 13 and the hottest atom in slab 1 were exchanged every 50 fs, which formed an effective thermal flux of ~3.50 eV/ps between the slabs 1 and 13.

**References**


[1] Y.-S. Song, J. Kim, and S.-H. Jhi, Phonon Instability and Broken Long-Ranged *p* Bond in Ge-Sb-Te Phase-Change Materials from First Principles, *Phys. Rev. Appl.* **9**, 054044 (2018).

[2] Y. M. Beltukov, C. Fusco, A. Tanguy, and D. A. Parshin, Transverse and longitudinal vibrations in amorphous silicon, *J. Phys.: Conf. Ser.* **661**, 012056 (2015).

[3] F. Müller-Plathe, A simple nonequilibrium molecular dynamics method for calculating the thermal conductivity, *J. Chem. Phys.* **106**, 6082-6085 (1997).

[4] A. P. Thompson, H. M. Aktulga, R. Berger, D. S. Bolintineanu, W. M. Brown, P. S. Crozier, P. J. in 't Veld, A. Kohlmeyer, S. G. Moore, T. D. Nguyen*, et al.*, LAMMPS - a flexible simulation tool for particle-based materials modeling at the atomic, meso, and continuum scales, *Comput. Phys. Commun.* **271**, 108171 (2022).

[5] P. Virtanen and R. Gommers and T. E. Oliphant and M. Haberland and T. Reddy and D. Cournapeau and E. Burovski and P. Peterson and W. Weckesser and J. Bright*, et al.*, SciPy 1.0: fundamental algorithms for scientific computing in Python, *Nat. Methods* **17**, 261-272 (2020).

[6] H.-K. Lyeo, D. G. Cahill, B.-S. Lee, J. R. Abelson, M.-H. Kwon, K.-B. Kim, S. G. Bishop, and B.-k. Cheong, Thermal conductivity of phase-change material $Ge_2Sb_2Te_5$, *Appl. Phys. Lett.* **89**, 151904 (2006).

[7] J. Lee, E. Bozorg-Grayeli, S. Kim, M. Asheghi, H. S. Philip Wong, and K. E. Goodson, Phonon and electron transport through $Ge_2Sb_2Te_5$ films and interfaces bounded by metals, *Appl. Phys. Lett.* **102**, 191911 (2013).

[8] E. K. Kim, S. I. Kwun, S. M. Lee, H. Seo, and J. G. Yoon, Thermal boundary resistance at $Ge_2Sb_2Te_5$/ZnS:$SiO_2$ interface, *Appl. Phys. Lett.* **76**, 3864-3866 (2000).

[9] C. Peng, L. Cheng, and M. Mansuripur, Experimental and theoretical investigations of laser-induced crystallization and amorphization in phase-change optical recording media, *J. Appl. Phys.* **82**, 4183-4191 (1997).

[10] D. Campi, L. Paulatto, G. Fugallo, F. Mauri, and M. Bernasconi, First-principles calculation of lattice thermal conductivity in crystalline phase change materials: GeTe, $Sb_2Te_3$, and $Ge_2Sb_2Te_5$, *Phys. Rev. B* **95**, 024311 (2017).
